# Supplementary material for: Design and Control of a Small Humanoid Equipped with Flight Unit and Wheels for Multimodal Locomotion
Source: arXiv:2303.14718 source file (2024-03-09)
Supplement: Supplementary file 1 [file appendix.tex]

\section*{APPENDIX}

Appendixes should appear before the acknowledgment.
